# Supplementary material for: Event-Frame Fusion for Inter-Frame Segmentation via Event-Guided Motion
Source: arXiv:2609.22500 source file (2026-11-30)
Supplement: Supplementary file 1 [file X_suppl.tex]

\clearpage
\setcounter{page}{1}
\maketitlesupplementary


% \section{Rationale}
% \label{sec:rationale}
% % 
% Having the supplementary compiled together with the main paper means that:
% % 
% \begin{itemize}
% \item The supplementary can back-reference sections of the main paper, for example, we can refer to \cref{sec:intro};
% \item The main paper can forward reference sub-sections within the supplementary explicitly (e.g. referring to a particular experiment); 
% \item When submitted to arXiv, the supplementary will already included at the end of the paper.
% \end{itemize}
% % 
% To split the supplementary pages from the main paper, you can use \href{https://support.apple.com/en-ca/guide/preview/prvw11793/mac#:~:text=Delete%20a%20page%20from%20a,or%20choose%20Edit%20%3E%20Delete).}{Preview (on macOS)}, \href{https://www.adobe.com/acrobat/how-to/delete-pages-from-pdf.html#:~:text=Choose%20%E2%80%9CTools%E2%80%9D%20%3E%20%E2%80%9COrganize,or%20pages%20from%20the%20file.}{Adobe Acrobat} (on all OSs), as well as \href{https://superuser.com/questions/517986/is-it-possible-to-delete-some-pages-of-a-pdf-document}{command line tools}.

\section{Difference motion estimation and OF }.
\begin{figure*}
    \centering
    \includegraphics[width=\linewidth]{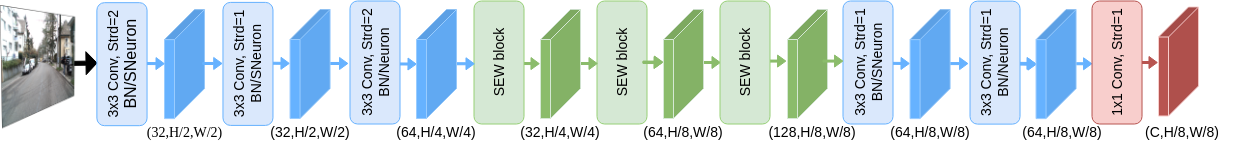}
    \caption{Detailed architecture of SegSNet. "Strd" denotes the stride applied in each convolutional layer, H and W represent the input’s height and width and C the number of segmentation classes. SEW refers to the residual Spike-Element-Wise blocks. The final output layer is referred to as logits.}
    \label{fig:segsnet}
\end{figure*}

\begin{figure*}
    \centering
    \includegraphics[width=0.7\linewidth]{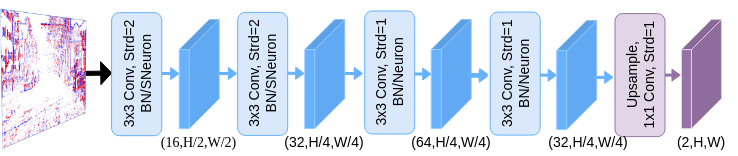}
    \caption{Detailed architecture of SegMoSNet. "Strd" denotes the stride applied in each convolutional layer, and H and W indicate the input’s height and width. The upsampling operation is performed using bilinear interpolation.}
    \label{fig:segmosnet}
\end{figure*}

In our approach, we draw inspiration from video segmentation techniques that utilize optical flow. Nevertheless, given the challenges related to accurate optical flow prediction discussed in Sec.~\ref{intro}, we substitute it with motion prediction estimation. It is important to clearly distinguish between these two concepts. Let $I_0, I_1$ be two consecutive frames acquired at $t_0$ and $t_1$, $M_0$ (resp. $M_1$) the semantic segmentation at $t_0$ (resp. $t_1$) and $W_f(\cdot)$ denote warping by a flow field $f$. Optical flow is typically learned by minimizing a reconstruction or photometric loss over images :
\begin{equation}\label{flow}
f^\star_{\text{flow}} = \arg\min_f \mathcal{L}_{\text{flow}}(f; I_0, I_1)
\end{equation}
In contrast, our motion estimation network is trained to minimize a segmentation-specific objective:
\begin{equation}
f^\star_{\text{motion}} = \arg\min_f \mathcal{L}_{\text{seg}}\big(W_f(M_0), M_1\big)
\end{equation}
which encourages the predicted flow to transport semantic masks consistently across time. In other words, optical flow emphasizes pixel-wise accuracy, while our motion estimation emphasizes semantic consistency, a difference we highlight further in an ablation study at the end of this chapter, contrasting both approaches.  

\section{Method description}
\subsection{Networks details}
The detailed architectures of our SNN-based segmentation (SegSNet) and motion estimation (SegMoSNet) networks are shown in Fig.~\ref{fig:segsnet} and Fig.~\ref{fig:segmosnet}, respectively. The segmentation mask, which assigns a class label to each pixel, is obtained by applying the argmax operation to the output layer of SegSNet, referred to as logits.
\subsection{Warping function}
The warping function used in our approach to propagate the segmentation logits $S_{i,k}$ of the $k^{th}$ inter-frame segmentation, generated between consecutive frames $I_i$ and $I_{i+1}$, based on the observed motion within $\Delta t$, is defined as follows:

\begin{equation} \label{warp}
S_{i,k+1}^C(p) = \sum_q G(q, p+\delta p) S_{i,k}(q)
\end{equation}

Here,t $k$ refers to the number of the inter-frame segmentation with $k=0$ referring to the segmentation of $I_i$. $C$ indexes the number of classes and $q$ enumerates spatial positions in the logits. The variable $p$ represents a pixel location in $S_{i,k+1}$, while $p + \delta p$ corresponds to its source location in $S_{i,k}$, with $\delta p$ indicating the motion estimation of $p$ within $\Delta t$. The bilinear interpolation kernel $G(q, p+\delta p)$ weights the contribution of each neighboring pixel $q$ and is expressed as the product of two one-dimensional kernels:

\begin{equation}
G(q, p+\delta p) = g(q_x, p_x+\delta p_x) \cdot g(q_y, p_y+\delta p_y) 
\end{equation}
with $\quad g(a,b) = \max(0, 1 - |a-b|)$.


\subsection{Recurrent structure representation}

Fig.~\ref{unfold} illustrates the recurrent structure of SegMoSNet. The membrane potential 
\( U_{\mathbb{T}_i}^{l_j} \) of a neuron in layer \( l_j \) at timestep \( \mathbb{T}_i \) is computed by combining the previous membrane potential with the spikes \( S_{\mathbb{T}_i}^{l_j} \) triggered at the previous timestep such that, if a spike occurred in that timestep, the membrane potential is reset (horizontal lines). Additionally, inputs from the previous layer are considered: when a neuron in the preceding layer fires, the corresponding synapse is activated, and its weight \( W_{l_{j-1}} \) is applied (vertical lines). Note that it shows the neurons of the first two layers. 
\begin{figure}[t]
    \centering
    \includegraphics[width=0.35\linewidth]{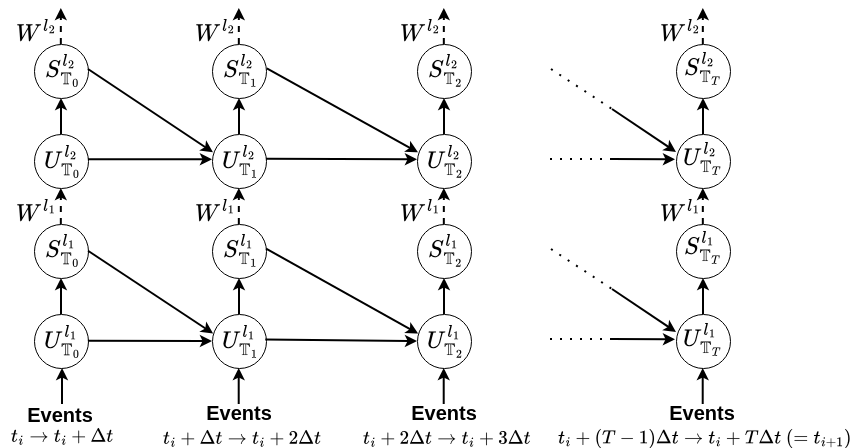}
    \caption{Recurrent structure representation of SegMoSNet}
    \label{unfold}
\end{figure}

\section{Energy measurement}
Following \cite{kim_beyond_2021}, \cite{nitin_rathi_diet-snn_2020} and \cite{zhang_accurate_2024}, we compute the number of ACC operations performed by an SNN in layer $l$ using the same formulation as in these works: :  
\begin{equation}
\text{ACC}_{l} = FR_l \times T \times A_l,
\end{equation}
where $FR_l$ is the mean firing rate over the testset, defined as
\begin{equation}
FR_l = \frac{\# \text{spikes in layer } l}{\# \text{neurons in layer } l},
\end{equation}
$T$ denotes the number of timesteps, which we set to $1$ since inference is performed using a single timestep and $A_l$ is the number of addition operations in the layer $l$, given by: 
\begin{equation}
A_l = k^2 \times H_{\text{out}} \times W_{\text{out}} \times C_{\text{in}} \times C_{\text{out}}
\end{equation}
where $k$ is the kernel size, $H_{\text{out}}$ and $W_{\text{out}}$ are the output feature map dimensions and $C_{\text{in}}$ and $C_{\text{out}}$ are the numbers of input and output channels, respectively.

Although SNNs primarily rely on additions, multiplications are still required in the input layer to process integer or floating-point inputs. Therefore, the multiplication count for this layer is set equal to the corresponding $A_l$ value ($MAC_{Input}=A_l$, with $l$ is the input layer). 

For energy estimation, we adopt the widely used 45nm CMOS values \cite{horowitz_11_2014}: $0.9$pJ per ACC and $4.6$pJ per MAC and compute the energy as: 
\begin{equation}
\text{Energy}_{\text{SNN}} = \sum_l \text{ACC}_l \times 0.9 + \text{MAC} \times 4.6 
\end{equation}

It is important to note that the current measurements consider only synaptic operations. A more comprehensive evaluation could also account for memory access, as proposed in Lemaire et al. \cite{lemaire_analytical_2023} and Damphofer et al. \cite{pimenidis_investigating_2022} which would provide a more realistic estimate of the overall computational cost.


\section{Ablation study}
\subsection{Why not optical flow?}
Table~\ref{tab:ablation_of} reports both the MIoU and runtime on the test set, comparing our method (SegMoSNet) with IDNet, evaluated at every frame. The results are consistent with ~\cref{fig:miou_vs_epe}, showing that SegMoSNet achieves higher MIoU than the optical flow–based approach at both $100$Hz (predictions every $10$ms) and $200$Hz (predictions every $5$ms). In addition, SegMoSNet is significantly more efficient, running over two orders of magnitude faster than IDNet on both GPU and CPU.
% \begin{table}[]
% \centering
% \begin{tabular}{l@{\hskip 6pt}c@{\hskip 6pt}c@{\hskip 6pt}}
% \toprule
%  & 100Hz & 200Hz \\ 
%  \midrule
%  Motion-based (Ours)  & 56.12\%  & 55.76\% \\ 
%  \midrule
%  \multirow{2}{*}{OF-based (IDNet)}  & 55.11\%  & 54.13\% \\ 
%                                 & (-0.16) & (-1.63)\\ 
                                
% \bottomrule
% \end{tabular}
% \caption{Results on the test set at $100$Hz and $200$Hz using our motion estimation network (SegMoSNet) and the optical flow network (IDNet) \cite{wu_lightweight_2024}. The values in parentheses indicate the performance drop of the IDNet-based approach compared to SegMoSNet.}
% \label{tab:ablation_of}
% \end{table}
\begin{table}[b]
\centering
\begin{tabular}{l@{\hskip 6pt}c@{\hskip 6pt}c@{\hskip 6pt}cc}
\toprule
 & \multicolumn{2}{c}{MIoU} & \multicolumn{2}{c}{Runtime (ms)} \\
\cmidrule(lr){2-3} \cmidrule(lr){4-5}
 & 100Hz & 200Hz & GPU & CPU \\ 
\midrule
Motion-based (Ours)  & 56.12\%  & 55.76\% & 1.18 & 13.96 \\ 
\midrule
\multirow{2}{*}{OF-based (IDNet)}  & 55.11\%  & 54.13\% & 122 & 1350 \\ 
                                   & (-0.16) & (-1.63) & ($\times103$) & $(\times96.70)$ \\ 
\bottomrule
\end{tabular}
\caption{Comparison of segmentation accuracy (MIoU) at $100$Hz and $200$Hz, along with the average runtime per inference, between our motion estimation network (SegMoSNet) and the optical flow–based network (IDNet) \cite{wu_lightweight_2024} on the test set. Values in parentheses in the MIoU column indicate the performance drop of IDNet relative to SegMoSNet, while those in the runtime column show the speed-up factor of SegMoSNet compared to IDNet.}
\label{tab:ablation_of}
\end{table}
\subsection{Dice loss}
To evaluate the contribution of the Dice function within our global loss, we analyze the per-class MIoU both with and without it. As indicated in Table \ref{dice}, incorporating the Dice function noticeably improves segmentation accuracy, yielding an overall MIoU increase of $2.02\%$. This improvement is especially pronounced in underrepresented classes: \textit{pedestrian} and \textit{traffic sign} classes see substantial gains of $7.80\%$ and $10.11\%$, respectively. Meanwhile, classes such as \textit{sidewalk}, \textit{fence} and \textit{pole} also experience moderate segmentation enhancements, averaging around $2\%$.
\clearpage
\clearpage
\twocolumn[
\begin{center}
\scriptsize
\begin{tabular}{l@{\hskip 2pt}c@{\hskip 3pt}c@{\hskip 3pt}c@{\hskip 3pt}c@{\hskip 3pt}c@{\hskip 3pt}c@{\hskip 3pt}c@{\hskip 3pt}c@{\hskip 3pt}c@{\hskip 3pt}c@{\hskip 3pt}c|@{\hskip 3pt}c@{\hskip 3pt}c@{\hskip 10pt}}
\toprule
        &  Background &  Building &  Fence   &  Pedestrian  &  Pole    &  Road    &  Sidewalk &  Vegetation &  Car     &  Wall    &  Traffic sign & Mean \\ \midrule                                                                                                                                                                
CE      &  94.54 & 80.38 & 16.73 & 15.81 & 20.08 & 92.59 & 63.33 & 85.72 & 74.70 & 23.30 & 29.80 & 54.27\\ \midrule
\multirow{2}{*}{CE+Dice} & 94.41 & 80.31 & \textbf{19.14 }& \textbf{23.61} & \textbf{22.92} & 92.68 & \textbf{64.70} & 84.99 & \textbf{74.73} & 21.75 & \textbf{39.91} & 56.29 \\
                         & (-0.13) & (-0.07) & (+2.41) & (+7.80) & (+2.85) & (+0.09) & (+1.36) & (-0.73) & (+0.03) & (-1.55) & (+10.11) & (+2.02)\\
\bottomrule
\end{tabular}
\captionof{table}{Comparison of per-class MIoU on the DSEC-Semantic dataset between models trained with Cross-Entropy (CE) loss and a combination of CE and Dice loss. Values in brackets indicate the relative change of CE+Dice compared to CE.}
\label{dice}
\end{center}
]
